# Supplementary material for: Ouroboros3D: Image-to-3D Generation via 3D-aware Recursive Diffusion
Source: arXiv:2406.03184 source file (2025-05-01)
Supplement: Supplementary file 1 [file X_suppl.tex]

\clearpage
\setcounter{page}{1}
\maketitlesupplementary

\section{Supplementary}

\subsection{Video Model Fine-tuning}
\label{videomodel}
Based on the approach outlined in SVD, the generation process employs the EDM framework. Let $p_{\text{data}}(\mathbf{x}_0)$ represent the video data distribution, and $p(\mathbf{x}; \sigma)$ be the distribution obtained by adding Gaussian noise with variance $\sigma^2$ to the data. For sufficiently large $\sigma_{\text{max}}$, $p(x; \sigma_{\text{max}}^2)$ approximates a normal distribution $\mathcal{N}(0, \sigma_{\text{max}}^2)$. Diffusion models (DMs) leverage this property and begin with high variance Gaussian noise, $x_M \sim \mathcal{N}(0, \sigma_{\text{max}}^2)$, and then iteratively denoise the data until reaching $\sigma_0 = 0$.

In practice, this iterative refinement process can be implemented through the numerical simulation of the Probability Flow ordinary differential equation (ODE):
\begin{equation}
d\mathbf{x} = -\dot{\sigma}(t)\sigma(t)\nabla_\mathbf{x} \log p(\mathbf{x}; \sigma(t)) \, dt
\end{equation}
where $\nabla_\mathbf{x} \log p((\mathbf{x}; \sigma)$ is called as score function. 

DM training is to learn a model $s_\theta(\mathbf{x}; \sigma)$ to approximate the score function $\nabla_\mathbf{x} \log p((\mathbf{x}; \sigma)$. The model can be parameterized as:
\begin{equation}
\nabla_\mathbf{x} \log p((\mathbf{x}; \sigma) \approx s_\theta((\mathbf{x}; \sigma) = \frac{D_\theta(\mathbf{x}; \sigma) - \mathbf{x}}{\sigma^2},
\end{equation}
where $D_\theta$ is a learnable denoiser that aims to predict ground truth $\mathbf{x}_0$. 

The denoiser $D_\theta$ is trained via denoising score matching (DSM):
\begin{equation}
\mathbb{E}_{\mathbf{x}_0 \sim p_{\text{data}}(\mathbf{x}_0), (\sigma,n) \sim p(\sigma,n)} \left[ \lambda_\sigma \| D_\theta(\mathbf{x}_0 + n; \sigma) - \mathbf{x}_0 \|_2^2 \right],
\end{equation}
where $p(\sigma, n) = p(\sigma) \mathcal{N}(n; 0, \sigma^2)$, $p(\sigma)$ is a distribution over noise levels $\sigma$, $\lambda_\sigma$ is a weighting function. The learnable denoiser $D_\theta$ is parameterized as:
\begin{equation}
D_\theta(\mathbf{x}; \sigma) = c_{\text{skip}}(\sigma)\mathbf{x} + c_{\text{out}}(\sigma)F_\theta(c_{\text{in}}(\sigma)\mathbf{x}; c_{\text{noise}}(\sigma)),
\end{equation}
where $F_\theta$ is the network to be trained.

We sample $\log\sigma \sim \mathcal{N}(P_{\text{mean}}, P_{\text{std}}^2)$, with $P_{\text{mean}} = 1.0$ and $P_{\text{std}} = 1.6$. Then we obtain all the parameters as follows:
\begin{equation}
    c_{\text{in}} = \frac{1}{\sqrt{\sigma^2+1}}
\end{equation}
\begin{equation}
    c_{\text{out}} = \frac{-\sigma}{\sqrt{\sigma^2+1}}
\end{equation}
\begin{equation}
    c_{\text{skip}}(\sigma) = \frac{1}{\sigma^2+1}
\end{equation}
\begin{equation}
    c_{\text{noise}}(\sigma) = 0.25 \log \sigma
\end{equation}
\begin{equation}
    \lambda(\sigma) = \frac{1+\sigma^2}{\sigma^2}
\end{equation}

We fine-tune the network backbone $F_\theta$ on multi-view images of size $512 \times 512$. During training, for each instance in the dataset, we uniformly sample 8 views and choose the first view as the input view.
view images of size $512\times 512$.

\subsection{Canonical Coordinates Map}
\label{coordinates_map}

\begin{figure}[h]
    \centering
    \includegraphics[width=0.5\linewidth]{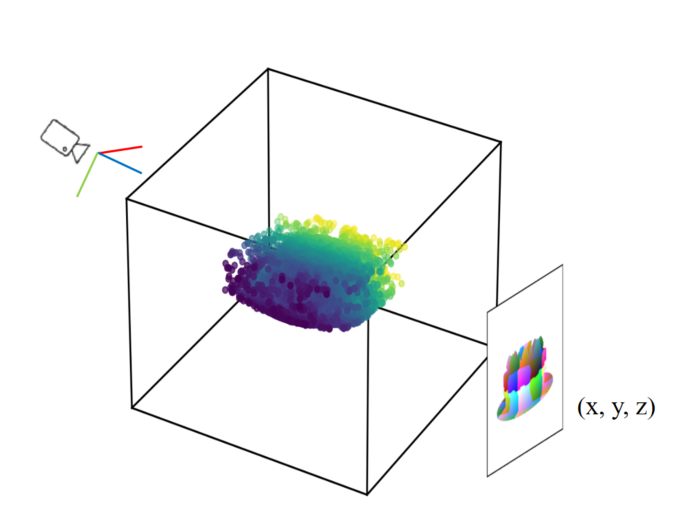}
    \caption{The projection process of coordinates map.}
    \label{fig:enter-label}
\end{figure}

For control networks of image diffusion models, the conditional maps like depth maps need to be normalized to [0, 1], typically using the formula: \((p - p_{mean}) / (p_{max} - p_{min})\). For multi-view generation, each view performs a normalize operation on itself, which results in a scale ambiguity. At the same time, the depth map is relative to a certain view, and the correlation between the depth values is not significant across views.

To avoid the above issues caused by self-normalization, we use canonical coordinate maps (CCM). Coordinate maps transform the depth value \(d\) to a common world coordinate system using the camera's intrinsic and extrinsic parameters, represented as \((X, Y, Z)\). The transformation formula is:
\[ \begin{pmatrix} X \\ Y \\ Z \end{pmatrix} = K^{-1} \cdot \begin{pmatrix} u \\ v \\ 1 \end{pmatrix} \cdot d \]
where \((u, v)\) are the pixel coordinates, \(d\) is the corresponding depth value, and \(K\) is the camera intrinsic matrix.
Then the coordinate values of all views will be multiplied by a \textbf{global} scale and added an offset value to convert to the range of 0 to 1. This representation makes the correlation between different views more significant and is helpful for multi-view generation.

\subsection{Algorithm}
\label{app:algorithm}
\begin{algorithm}[H]
\caption{Training}
\label{alg:train_loss}
\KwIn{x, cond\_image, cameras, timestep}
\KwOut{loss}
// Returns the loss on a training example x. Details about EDM are omitted here.

\Begin{
    noise $\leftarrow$ Sample from Normal Distribution\;

    noisy\_x $\leftarrow$ Add\_Noise(x, noise, timestep)\;

    pred\_x $\leftarrow$ $F$(noisy\_x, cond\_image, timestep, cameras)\;

    pred\_i $\leftarrow$ VAE\_Decoder(pred\_x)\;

    self\_cond $\leftarrow$ $\mathcal{G}$(pred\_i, cameras, timestep)\;

    \If{Random\_Uniform(0, 1) > 0.5}{
    
        pred\_x $\leftarrow$ F(noisy\_x, cond\_image, timestep, cameras, self\_cond)\;
    }

    loss\_mv $\leftarrow$ MSE\_Loss(pred\_x, x)\;

    loss\_recon $\leftarrow$ MSE\_Loss(self\_cond, x) + LPIPS\_Loss(self\_cond, x)\;

    loss $\leftarrow$ loss\_mv + loss\_recon\;

    \Return{loss}
}
\end{algorithm}

\begin{algorithm}[H]
\caption{Inference}
\label{alg:inference}
\KwIn{cond\_image, cameras, timesteps}
\KwOut{images, 3d\_model}
// Generate multi-view images and 3D model from a condition image.

\Begin{
    self\_cond $\leftarrow$ None\;
    
    x\_t $\leftarrow$ Sample from Normal Distribution\;
    
    \ForEach{timestep in timesteps}{
    
        pred\_x $\leftarrow$ $F$(x\_t, cond\_image, timestep, cameras, self\_cond)\;
        
        pred\_i $\leftarrow$ VAE\_Decoder(pred\_x)\;
        
        self\_cond $\leftarrow$ $\mathcal{G}$(pred\_i, cameras, timestep)\;
        
    }
    
    \Return{pred\_i, self\_cond}
}
\end{algorithm}

\subsection{3D-aware Feedback}
\label{app: 3dfeedback}
% \begin{figure}
%     \centering
%     \includegraphics[width=0.25\linewidth]{fig/resblock.png}
%     \caption{Architecture of the residual block used in Feedback Stage.}
%     \label{resblock}
% \end{figure}

% \begin{table}[h]
%     \centering
%     \begin{tabular}{cc}
%         \toprule
%        Input & $\text{inp} \in \mathbb{R}^{ 3 \times 512\times 512}$ \\
%         \midrule
%         PixelShuffle\citep{pixelshuffle2016} & $ 192\times 64 \times 64$ \\
%         ResBlock $\times 3$ & $ 320\times 64 \times 64$ \\
%         ResBlock $\times 3$ & $ 640\times 32 \times 32$ \\
%         ResBlock $\times 3$ & $ 1280\times 16 \times 16$ \\
%         ResBlock $\times 3$ & $ 1280\times 8 \times 8$ \\
%         \bottomrule
%     \end{tabular}
%     \caption{Comparison of performance metrics.}
%     \label{resnetwork}
% \end{table}
    \begin{figure}[!ht]
    \begin{minipage}[b]{0.3\linewidth}
        \centering
        \includegraphics[width=0.6\linewidth]{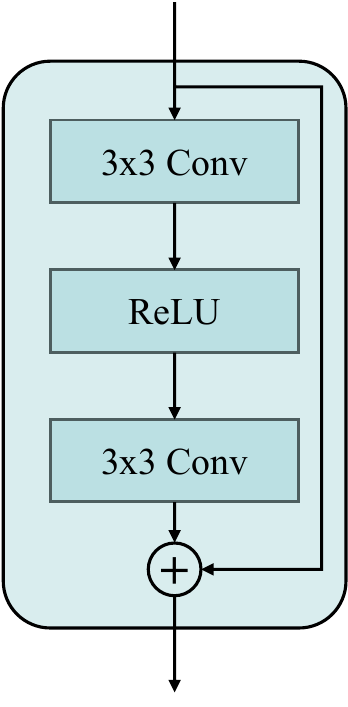}
        \caption{Architecture of the residual block used in the feedback stage.}
        \label{resblock}
    \end{minipage}
    \hfill
    \begin{minipage}[b]{0.7\linewidth}
        \centering
        \begin{table}[H]\footnotesize
            \caption{The detailed structure of all layers in the feedback injection network.}
            \label{resnetwork}
            \begin{tabular}{cc}
                \toprule
                Input & $\text{inp} \in \mathbb{R}^{3 \times 512 \times 512}$ \\
                \midrule
                PixelUnshuffle & $192 \times 64 \times 64$ \\
                ResBlock $\times 3$ & $320 \times 64 \times 64$ \\
                ResBlock $\times 3$ & $640 \times 32 \times 32$ \\
                ResBlock $\times 3$ & $1280 \times 16 \times 16$ \\
                ResBlock $\times 3$ & $1280 \times 8 \times 8$ \\
                \bottomrule
            \end{tabular}
        \end{table}
    \end{minipage}
\end{figure}

% \begin{table}[h]
% \centering
% \begin{tabular}{ccc}
% \toprule
% \textbf{Input} $\text{inp} \in \mathbb{R}^{ 3 \times 512\times 512}$ \\
% PixelShuffle  
% ResBlock $\times 3$ $17$
% \midrule
% \begin{tabular}{ccc}
% \textbf{Res Block} 
% \end{tabular} \\
% \toprule
% \end{tabular}
% \caption{All layers of }
% \end{table}

\cref{resblock} and \cref{resnetwork} provide a detailed illustration of the feedback injection netwrok. We use two networks to inject the coordinates map and RGB texture map feedback into the score function. Each network consists of four feature extraction blocks and three downsample blocks to adjust the feature resolution. The reconstruction coordinates map and RGB texture map initially have a resolution of \(512 \times 512\). We employ the pixel unshuffle operation to downsample these maps to \(64 \times 64\).

At each scale, three residual blocks are used to extract the multi-scale feedback features, denoted as \(F_P = \{F^1_p, F^2_p, F^3_p, F^4_p\}\) and \(F_T = \{F^1_t, F^2_t, F^3_t, F^4_t\}\) for the coordinates map and RGB texture map, respectively. These feedback features match the intermediate features \(F_{\text{enc}} = \{F^1_{\text{enc}}, F^2_{\text{enc}}, F^3_{\text{enc}}, F^4_{\text{enc}}\}\) in the encoder of the UNet denoiser. The feedback features \(F_P\) and \(F_T\) are added to the intermediate features \(F_{\text{enc}}\) at each scale as described by the following equations:

\begin{equation}
    \mathbf{F}_p = \mathcal{F}^0(P)
\end{equation}
\begin{equation}
    \mathbf{F}_t = \mathcal{F}^1(T)
\end{equation}
\begin{equation}
    \mathbf{F}^i_{\text{enc}} = \mathbf{F}^i_{\text{enc}} + \mathbf{F}_p^i + \mathbf{F}_t^i, \quad i \in \{1, 2, 3, 4\}
\end{equation}

where \(P\) represents the coordinates map feedback input, and \(T\) represents the RGB texture feedback input. \(\mathcal{F}^0\) and \(\mathcal{F}^1\) denote the functions of the feedback inject network applied to the coordinates map and RGB texture map, respectively.

\begin{figure}[h]
    \centering
    \includegraphics[width=0.5\textwidth]{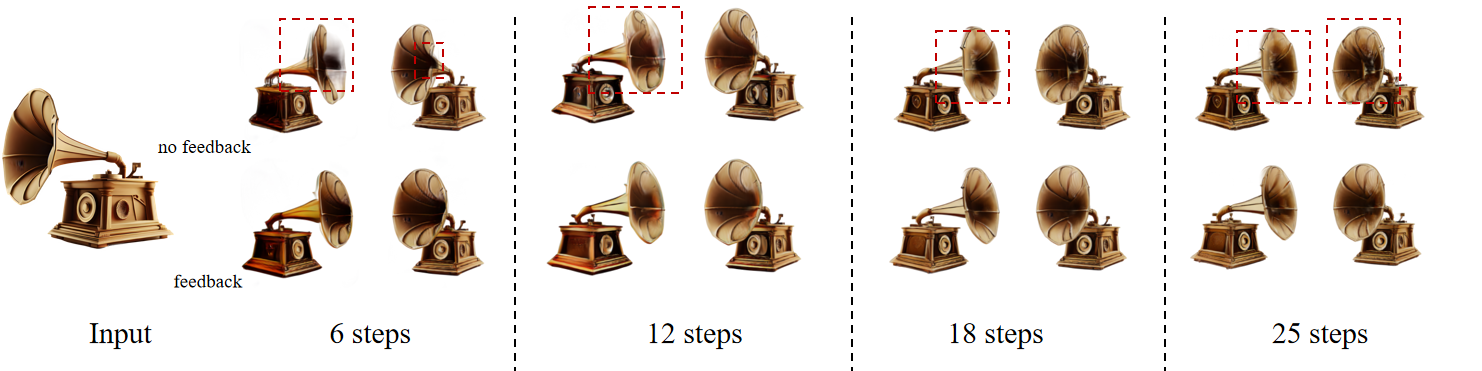}
    \caption{Visualization of the reconstruction results at different denoising steps. The process initially generates floaters and distorted geometries, but progressively refines them into cleaner representations. Through feedback mechanisms, the model optimizes shape and texture features in the early stages }
    \label{fig:visual}
\end{figure}

\subsection{visualization of denoising steps}
We visualize the reconstruction process at different denoising steps in \cref{fig:visual}. Early stages show floating artifacts and distorted geometries due to multi-view inconsistency. As denoising progresses, our recursive diffusion method gradually refines both the geometric accuracy and material properties of the reconstruction. By comparing the visual results, we observed that the 3D feedback mechanism achieved superior performance compared to the no-feedback condition.
